# Supplementary material for: A Language Agent for Autonomous Driving
Source: arXiv:2311.10813 source file (2024-07-28)
Supplement: Supplementary file 1 [file 0_system.tex]

\section{System Overview}

% include a graph capturing the whole working flow of our system.
